# Supplementary material for: Handling Neumann and Robin boundary conditions in a fictitious domain volume penalization framework
Source: arXiv:2101.02806 source file (2021-10-10)
Supplement: Supplementary file 1 [file Supplementary_Material.tex]

MATLAB scripts to simulate 1D Poisson problems of Sec.~\ref{sec_1d_same_flux_bc} and~\ref{sec_1d_different_flux_bc} are included in the supplementary material section. A MATLAB script used to generate signed distance functions for the complex domains considered
in Sec.~\ref{sec_complex_shapes} is also included.  The two dimensional test problems considered in this work can be obtained from the IBAMR Github repository~\cite{IBAMR-web-page}.
